# Supplementary material for: Cumulative neutrino background from quasar-driven outflows
Source: arXiv:1607.06476 source file (2016-09-22)
Supplement: Supplementary file 1 [file supplemental.pdf]

# Supplemental Material

---

**Hydrodynamical model of quasar-driven outflows.** The equations governing the hydrodynamics of quasar outflows are discussed in our companion paper, and are summarized as follows:

$$\frac{d^2 R_\mathrm{s}}{dt^2} = \frac{4\pi R_\mathrm{s}^2}{M_\mathrm{s}}(P_\mathrm{t} - P_0) - \frac{GM_\mathrm{tot}}{R_\mathrm{s}^2} - \frac{v_\mathrm{s}}{M_\mathrm{s}}\frac{dM_\mathrm{s}}{dt}\,, \tag{1a}$$

$$\frac{dM_\mathrm{s}}{dt} = 4\pi\rho_\mathrm{g} R_\mathrm{s}^2 v_\mathrm{s}\,, \tag{1b}$$

$$\frac{dP_\mathrm{t}}{dt} = \frac{\Lambda}{2\pi R_\mathrm{s}^3} - 5P_\mathrm{t}\frac{v_\mathrm{s}}{R_\mathrm{s}}\,, \tag{1c}$$

$$\Lambda = L_\mathrm{in} - L_\mathrm{cool}, \tag{1d}$$

where $M_\mathrm{s}$ is the swept-up mass of the outflowing shell, $M_\mathrm{tot}$ is the total gravitational mass and $P_\mathrm{t}$, $P_0$ are the thermal pressure in the shocked wind and ambient medium, respectively. The heating/cooling function $\Lambda$ includes continuous energy injection into the medium, $L_\mathrm{in}$ and cooling luminosity $L_\mathrm{cool}$, composed of free-free emission, synchrotron cooling, inverse Compton scattering and proton cooling.

We assume a spherical geometry for the gas density distribution and the galaxy mass profile for simplicity. The density profile of the surrounding gas can be described by a broken power-law:

$$\rho_\mathrm{g}(R) \propto \begin{cases} R^{-\alpha} & (R < R_\mathrm{disk}) \\ R^{-\beta} & (R_\mathrm{disk} < R < R_\mathrm{vir}) \end{cases} \tag{2}$$

where $\alpha$ and $\beta$ are power-law indices for the disk and halo components and $R_\mathrm{disk}$ and $R_\mathrm{vir}$ are the radius of the disk and halo, respectively.

**Neutrino spectrum.** Following Kelner et al. (2006), we use an analytical approximation for calculating the neutrino spectrum. The muonic neutrino spectrum $F_{\nu_\mu}$ is given by $F_{\nu_\mu} = F_{\nu_\mu^{(1)}} + F_{\nu_\mu^{(2)}}$, where $F_{\nu_\mu^{(1)}}$ corresponds to neutrinos produced through $\pi \to \mu\nu_\mu$,

$$F_{\nu_\mu^{(1)}}(x, E_\mathrm{p}) = B'\frac{\ln y}{y}\left[\frac{1 - y^{\beta'}}{1 + k' y^{\beta'}(1 - y^{\beta'})}\right]^4 \left[\frac{1}{\ln y} - \frac{4\beta' y^{\beta'}}{1 - y^{\beta}} - \frac{4k'\beta' y^{\beta'}(1 - 2y^{\beta'})}{1 + k' y^{\beta'}(1 - y^{\beta'})}\right]\,, \tag{3}$$

with $x = E_{\nu_\mu}/E_\mathrm{p}$ and $y = x/0.427$. Here,

$$B' = 1.75 + 0.204\ell + 0.010\ell^2\,, \tag{4}$$

$$\beta' = \left(1.67 + 0.111\ell + 0.0038\ell^2\right)^{-1}\,, \tag{5}$$

$$k' = 1.07 - 0.086\ell + 0.002\ell^2\,. \tag{6}$$

The muonic neutrino spectrum from the decay of muons $F_{\nu_\mu^{(2)}}$ can be described as:

$$F_{\nu_\mu^{(2)}}(x, E_\mathrm{p}) = -B_e \frac{\left[1 + k_e(\ln x)^2\right]^3}{x(1 + 0.3/x^{\beta_e})}(\ln x)^5\,, \tag{7}$$

where $x = E_e/E_\pi$. Here,

$$B_e = \left(69.5 + 2.65\ell + 0.3\ell^2\right)^{-1} \tag{8}$$

$$\beta_e = \left(0.201 + 0.062\ell + 0.00042\ell^2\right)^{-1/4} \ , \tag{9}$$

$$k_e = \frac{0.279 + 0.141\ell + 0.0172\ell^2}{0.3 + (2.3 + \ell)^2} \ . \tag{10}$$
